# Supplementary material for: Optimal Sets and Solution Paths of ReLU Networks
Source: arXiv:2306.00119 source file (2024-01-19)
Supplement: Supplementary file 1 [file conjectures.tex]

%!TEX root=../main.tex
\begin{proposition}\label{prop:proximal-gradient}
	The proximal-gradient algorithm with update rule
	\begin{equation}\label{eq:proximal-gradient}
		\begin{aligned}
			\wplus   & = \wk - \eta \nabla f(\w^k)                                          \\
			\w^{k+1} & =  \frac{\wplus}{\norm{\wplus}_2}(\norm{\wplus}_2 - \eta \lambda)_+,
		\end{aligned}
	\end{equation}
	and initialized at \( \w^0 \in \Row(X) \) converges to the min-norm solution \( \wmin(\lambda) \).
\end{proposition}
\begin{proof}
	The proof follows by showing that \( \w^{k} \in \Row(X) \)
	for all \( k \geq 0 \), which implies \( \w^{k}_\acts \in \Row(\Xas) \).
	As a result, the limit --- which is known to be a solution by standard
	optimization theory --- satisfies \( \lim_k \w^k \in \Row(\Xas) \).
	This condition uniquely identifies the min-norm solution,
	which yields the desired result.

	Assume that \( \w^k \in \Row(X) \) and observe that
	\[
		\wplus = \wk - \eta X^\top (X w - y),
	\]
	implies \( \wplus \in \Row(X) \) as well.
	Given \( \wplus \), \( \w^{k+1} \) is the unique solution to the following
	optimization problem
	\[
		\w^{k+1} =
		\argmin_{w} \cbr{
			\lambda \sum_{\bi \in \calB} \norm{\wi}_2 +
			\frac{1}{2\eta}\norm{\w - \wplus}_2^2.
		}
	\]
	Optimality conditions imply \( \w^{k+1} + \eta \lambda v = \wplus \),
	where \( \vi \in \lambda \partial \norm{\wi^{k+1}}_2 \).
	This immediately implies \( w^{k+1} + \eta \lambda v \in \Row(X) \).
	Now, suppose \( \w^{k+1} = a + b \), where \( a \in \Row(X) \) and
	\( b \in \Null(X) \).
	Clearly if \( \wi = 0 \), then \( b_\bi = 0 \) must also hold.
	If \( \wi \neq 0 \), then
	by definition of \( \partial \norm{\wi}_2 \), we have
	\[
		a_\bi + b_\bi + \eta \lambda \frac{a_\bi + b_\bi}{\norm{a_\bi + b_\bi}_2}
		= \wplus_\bi.
	\]
	The issue now is that \( a_\bi \) and \( b_\bi \) are not necessarily
	orthogonal; \( a_\bi \in \Row(\Xbi) \), but \( b_\bi \) is not necessarily in
	\( \Null(\Xbi) \).
	I am currently stuck here.
\end{proof}

\begin{lemma}
	Let \( \lambda > 0 \).
	and suppose the equicorrelation set is \( \equi \).
	Then the solution to the  dual problem
	is the same as the solution to
	\begin{equation}\label{eq:reduced-dual}
		\begin{aligned}
			\max_{\eta} \;
			 & - \half (\eta - X^\top y) (X^\top X)^+ (\eta - X^\top y) + \half \norm{y}_2^2                               \\
			 & \quad \quad \text{s.t.} \quad \eta \in \Row(X), \; \norm{\eta_\bi}_2 = \lambda \; \forall \; \bi \in \equi.
		\end{aligned}
	\end{equation}
\end{lemma}
\begin{proof}
	Let \( \eta^* \) be a solution to the dual problem
	and \( \eta' \) a solution to the dual problem with reduced constraints.
	Let \( d^* \) be the optimal value of the dual problem and \( d' \) the
	optimal value of the reduced problem.
	Observe that \( d' \geq d^* \) since \( \eta^* \) is feasible for the
	reduced problem.

	Assume that \( \eta'_\bi \geq \lambda \) for some \( \bi \in \calB \setminus \calE \).
	Since \( \eta^*_\bi < \lambda \), there exists \( \alpha > 0 \)
	such that
	\[
		\bar \eta = \alpha \eta^* + (1- \alpha) \eta',
	\]
	is feasible.
	Moreover, the objective obtained by \( \bar \eta \) satisfies
	\[
		- \half (\bar \eta - X^\top y) (X^\top X)^+ (\bar \eta - X^\top y) + \half \norm{y}_2^2                              \geq \alpha d' + (1 - \alpha) d^*,
	\]
	by concavity, which implies that \( \bar \eta \) is a solution to the dual problem.
	However, the dual solution to the dual problem is exactly the block correlation
	vector, which is unique.
	This is a contradiction, so we conclude that \( \eta' \) is feasible
	for the dual problem.
	Feasibility combined with \( d' \geq d^* \) implies \( d' = d^* \)
	and \( \eta' = \eta^* \).
\end{proof}

The KKT conditions for constraint reduced dual problem are
\begin{equation}\label{eq:dual-kkt-conditions}
	\begin{aligned}
		(X^\top X)^+ (\eta - X^\top y)
		+ (I - X X^+) \beta
		+ \sum_{\bi \in \equi} \alpha_\bi \frac{\wi}{\norm{\eta_\bi}_2}
		                               & = 0                                       \\
		(I - X X^+) \eta + X X^+ \beta & = 0                                       \\
		\norm{\wi}_2                   & = \lambda \quad \forall \; \bi \in \equi.
	\end{aligned}
\end{equation}

The Jacobian of this system is
\begin{equation}
	J =
	\begin{bmatrix}
		(X^\top X)^+ & (I - X X^+) & D(\eta) \eta \\
		(I - X X^+)  & X X^+       & 0            \\
		D(\eta) \eta & 0           & 0
	\end{bmatrix},
\end{equation}
where \( D(\eta) \) is a block-diagonal matrix with blocks given by
\( D_\bi(w) = I / \norm{\wi}_2 \) if \( \eta \in \equi \)
and \( D_\bi(w) = 0 \) otherwise.

\begin{proposition}
	The Jacobian of the constraint reduced problem is invertible
	for every \( \bar \eta, \bar \beta, \bar \alpha \).
\end{proposition}
\begin{proof}
	Suppose there exists \( \eta, \beta, \alpha \) such that
	\[
		\begin{bmatrix}
			(X^\top X)^+           & (I - X X^+) & D(\bar \eta) \bar \eta \\
			(I - X X^+)            & X X^+       & 0                      \\
			D(\bar \eta) \bar \eta & 0           & 0
		\end{bmatrix}
		\begin{bmatrix}
			\eta  \\
			\beta \\
			\alpha
		\end{bmatrix}
		= 0.
	\]
	For \( \we \)
\end{proof}

\begin{restatable}{proposition}{maxSupport}\label{prop:max-support}
	\textcolor{red}{WARNING: This result is out of date and cannot be relied on.}\\

	The min-norm solution is supported on \( \equi \) for almost
	every \( y \).
	As a result, \( \wmin \) has largest support (i.e most non-zero blocks) of
	any solution for almost every \( y \).
\end{restatable}
\begin{proof}
	By \cref{lemma:min-norm-expression},
	\[
		\wmin_{\equi} = (\Xe^\top \Xe)^+\sbr{\Xe^\top y - \ve(\lambda)},
	\]
	where \( \vi \in \lambda \partial \norm{\wi^*}_2 \) is the subgradient
	of the min-norm solution.
	As a result, we observe that a block in the equicorrelation set is zero
	if and only if
	\begin{equation}\label{eq:zero-entry}
		(\Xe^\top \Xe)^+_\bi \Xe^\top y  = (\Xe^\top \Xe)^+_\bi \ve(\lambda).
	\end{equation}
	Note that \( \norm{\vi}_2 = \lambda \) since \( \bi \in \equi \),
	meaning \( \norm{\ve}_2 = \lambda \sqrt{\abs{\equi}} \).
	As a result,
	\[
		\calS = \cbr{ (\Xe^\top \Xe)^+_\bi z :
			\norm{z}_2 = \lambda \sqrt{\abs{\equi}}
		},
	\]
	defines the shell of an ellipsoid which is strictly larger than the set of \( \ve(\lambda) \) vectors as \( y \) ranges over \( \R^n \).
	The inverse image of this shell under \( (\Xe^\top \Xe)^+_\bi \) is
	\[
		[(\Xe^\top \Xe)^+_\bi]^{-1} \calS
		= \cbr{z + x
			: \norm{z}_2 = \lambda \sqrt{\abs{\equi}},
			x \in \Null((\Xe^\top \Xe)^+_\bi)}
	\]
	The condition in \cref{eq:zero-entry} is equivalent to
	\[
		\Xe^\top y \in [(\Xe^\top \Xe)^+_\bi]^{-1} \calS.
	\]
	Splitting \( \Xe^\top y = c + d \), \( c \in \Row((\Xe^\top \Xe)^+_\bi) \)
	and \( d \in \Null((\Xe^\top \Xe)^+_\bi) \),
	the inclusion is satisfied when \( \norm{c}_2 = \lambda \sqrt{\abs{\equi}} \).
	This event is measure zero under any continuous probability distribution,
	which proves \( \wmin_\bi \neq 0 \) for almost every \( y \).

	We have shown that
	\( \wmin \) is supported on \( \equi \) for almost every \( y \).
	Since the largest support set any solution can have is \( \equi \),
	it holds that \( \wmin \) has the largest support of any solution
	for almost every \( y \).
\end{proof}
