# Supplementary material for: Optimal Sets and Solution Paths of ReLU Networks
Source: arXiv:2306.00119 source file (2024-01-19)
Supplement: Supplementary file 2 [file one_d.tex]

%!TEX root=../main.tex

\begin{proposition}\label{prop:1d-to-lasso}
	Let \( Z \in \R^{n \times 1} \) be a one-dimensional training set
	and \( y \in \R^n \) the associated targets.
	The two-layer ReLU training problem with unregularized bias,
	\begin{equation}\label{eq:1d-relu}
		\begin{aligned}
			\min_{w_1, w_2, b} \half \norm{\sum_{i=1}^m (Z w_{1i} + b_{1i})_+ w_{2i} + b_2 - y}_2^2
			+ \frac{\lambda}{2} \norm{w_1}^2_2 + \norm{w_2}_2^2,
		\end{aligned}
	\end{equation}
	is equivalent to the following Lasso problem:
	\begin{equation}\label{eq:1d-bi-dual}
		\min_{v, b} \half \norm{A v + b - y} + \lambda \norm{v}_1,
	\end{equation}
	where
	\[
		A =
		\begin{bmatrix}
			0         & 0         & \ldots & 0             & Z_n - Z_1       & Z_{n-1} - Z_1     & \ldots & Z_2 - Z_1 \\
			Z_2 - Z_1 & 0         & \ldots & 0             & \vdots          & \vdots            & \ddots & 0         \\
			Z_3 - Z_1 & Z_3 - Z_2 & \ldots & 0             & \vdots          & \vdots            & \ddots & 0         \\
			\vdots    & \vdots    & \ddots & \vdots        & Z_{n} - Z_{n-2} & Z_{n-1} - Z_{n-2} & \ldots & 0         \\
			\vdots    & \vdots    & \ddots & 0             & Z_{n} - Z_{n-1} & 0                 & \ldots & 0         \\
			Z_n - Z_1 & Z_n - Z_2 & \ldots & Z_n - Z_{n-1} & 0               & 0                 & \ldots & 0
		\end{bmatrix}
	\]
	Finally, solutions to the Lasso problem can be mapped to solutions of the
	non-convex program as follows:
	\begin{equation}
		w_{1i}, w_{2i}, b_{1i} =
		\begin{cases}
			\frac{|v_i|}{\sqrt{|v_i|}}, \text{sign}(v_i) \sqrt{|v_i|}, - Z_i \frac{|v_i|}{\sqrt{|v_i|}} & \mbox{if \( v_i \neq 0, i \leq n-1 \)} \\
			-\frac{|v_i|}{\sqrt{|v_i|}}, \text{sign}(v_i) \sqrt{|v_i|}, Z_i \frac{|v_i|}{\sqrt{|v_i|}}  & \mbox{if \( v_i \neq 0, i \leq n-1 \)} \\
			0, 0, 0                                                                                     & \mbox{otherwise.}
		\end{cases}
	\end{equation}
	and \( b_2 = b \) represents the bias in the Lasso problem.

\end{proposition}
\begin{proof}
	Following \citet{pilanci2020convexnn},
	we observe that \cref{eq:1d-relu} is equivalent to the following constrained
	problem:
	\begin{equation}
		\begin{aligned}
			\min_{w_1, w_2, b_1, b_2} & \half \norm{\sum_{i=1}^m (Z w_{1i} + b_{1i})_+ w_{2i} + b_2 - y}_2^2 + \lambda \norm{w_2}_1 \\
			                          & \hspace{5em} \text{ s.t. } w_{1i} \in \cbr{+1 , -1}.
		\end{aligned}
	\end{equation}
	Now we introducing the constraint \( a = \sum_{i=1}^m (Z w_{1i} + b_{1i})_+ w_{2i} + b_2 \)
	so that we may compute the dual problem,
	\begin{align*}
		p^* & = \min_{w_1, w_2, b_1, b_2, a}
		\half \norm{a - y}_2^2 + \lambda \norm{w_1}^2_2 + \norm{w_2}_2^2                                                                                                    \\
		    & \hspace{5em} \text{ s.t. } a = \sum_{i=1}^m (Z w_{1i} + b_{1i})_+ w_{2i} + b_2, \, w_{1i} \in \cbr{+1, -1}
		\intertext{
			Forming the Lagrangian and infimizing over the primal parameters,
		}
		d(\eta)
		    & = \min_{w_1, w_2, b_1, b_2, a} \half \norm{a - y}_2^2 + \abr{\eta, a}
		+ \abr{\eta, \sum_{i=1}^m (Z w_{1i} + b_{1i})_+ w_{2i} + b_2} + \lambda \norm{w_2}_1 + \mathbbm{1}_{\cbr{+1, -1}^m}(w_{1})                                          \\
		    & = \min_{w_1, w_2, b_1, b_2} \half \norm{\eta - y}_2^2 + \half \norm{y}^2_2
		+ \abr{\eta, \sum_{i=1}^m (Z w_{1i} + b_{1i})_+ w_{2i} + b_2} + \lambda \norm{w_2}_1 + \mathbbm{1}_{\cbr{+1, -1}^m}(w_{1})                                          \\
		    & = \min_{w_1, w_2, b_1} \half \norm{\eta - y}_2^2 + \half \norm{y}^2_2
		+ \abr{\eta, \sum_{i=1}^m (Z w_{1i} + b_{1i})_+ w_{2i}} + \lambda \norm{w_2}_1 + \mathbbm{1}_{\cbr{+1, -1}^m}(w_{1}) - \mathbbm{1}_{\{0\}}(\eta^\top \mathbbm{1})   \\
		    & = \min_{w_1, w_2, b_1} \half \norm{\eta - y}_2^2 + \half \norm{y}^2_2
		+ \abr{w_{2}, (Z w_{1}^\top + b_{1i} \mathbbm{1})_+ \eta} + \lambda \norm{w_2}_1 + \mathbbm{1}_{\cbr{+1, -1}^m}(w_{1}) - \mathbbm{1}_{\{0\}}(\eta^\top \mathbbm{1}) \\
		    & = \min_{w_1, b_1} \half \norm{\eta - y}_2^2 + \half \norm{y}^2_2
		- \mathbbm{1}(\norm{(Z w_{1}^\top + b_{1i} \mathbbm{1})_+ \eta}_\infty \leq \lambda) + \mathbbm{1}_{\cbr{+1, -1}^m}(w_{1}) - \mathbbm{1}_{\{0\}}(\eta^\top \mathbbm{1}).
	\end{align*}
	Minimizing over \( w_1 \) and \( b_1 \) in the last equation is equivalent
	to including linear semi-infinite constraints in the optimization problem,
	\begin{equation}\label{eq:1d-dual}
		\begin{aligned}
			d(\eta)
			 & =  \half \norm{\eta - y}_2^2 + \half \norm{y}^2_2              \\
			 & \hspace{2em} \text{ s.t. } \sup_{w_{1i} \in \cbr{+1, -1}^m, b}
			\abs{\eta^\top (Z w_{1i} + b_{1i} \mathbbm{1})_+} \leq \lambda.
		\end{aligned}
	\end{equation}
	Note that the number of neurons \( m \) vanishes since it is sufficient
	for one neuron to attain the maximum and define the constraint set.

	Let us analyze the constraint set.
	First, observe that we may remove \( w_{1i} \) by splitting it its
	possible values as follows:
	\[
		\cbr{ \eta :
			\sup_{w_{1i} \in \cbr{+1, -1}^m, b}
			\abs{\eta^\top (Z w_{1i} - b \mathbbm{1})_+}
			\leq \lambda
		}
		=
		\cbr{ \eta :
			\sup_{b}
			\abs{\eta^\top (Z - b \mathbbm{1})_+}
			\leq \lambda, \,
			\sup_{b}
			\abs{\eta^\top (Z - b \mathbbm{1})_-},
		}
	\]
	Consider first the optimization problem
	\[
		\sup_{b}
		\abs{\eta^\top (Z - b \mathbbm{1})_+}
	\]
	This is maximization of a piece-wise linear objective
	over pieces \( [-\infty, Z_{(1)}],  \cbr{[Z_{(j)}, Z_{(j+1)}]}_{j = 1}^n, [Z_{(n)}, \infty] \).
	Since the optimization is an LP over each piece, the optimum must occur
	in the set \( \cbr{- \infty, \infty} \cup \cbr{Z_{(j)}}_{j=1}^n \).
	Clearly it does not occur at \( \infty \).
	Taking \( b \rightarrow -\infty \), we deduce the constraint
	\( \eta^\top \mathbbm{1} = 0 \), otherwise the dual is infeasible.
	Under this constraint, the optimum must occur at one of the breakpoints.
	Enumerating over all such values of \( b \) gives the following:
	\begin{align*}
		\sup_{b}
		\abs{\eta^\top (Z - b \mathbbm{1})_+}
		 & =
		\sup_{j}
		\abs{\eta^\top (Z + Z_{(j)} \mathbbm{1})_+}.
		\intertext{
			Assuming without loss of generalizing that \( Z \) is sorted
			in increasing order, we obtain
		}
		 & = \norm{\eta^\top A_1}_\infty,
	\end{align*}
	where
	\[
		A_1 =
		\begin{bmatrix}
			0         & 0         & \ldots & 0             \\
			Z_2 - Z_1 & 0         & \ldots & 0             \\
			Z_3 - Z_1 & Z_3 - Z_2 & \ldots & 0             \\
			\vdots    & \vdots    & \ddots & 0             \\
			Z_n - Z_1 & Z_n - Z_2 & \ldots & Z_n - Z_{n-1}
		\end{bmatrix}
	\]
	A similar analysis gives
	\[
		\sup_{b}
		\abs{\eta^\top (Z - b \mathbbm{1})_-}
		=
		\norm{\eta^\top A_2}_\infty,
	\]
	where \( A_2 \) is
	\[
		A_2 =
		\begin{bmatrix}
			Z_n - Z_1     & Z_{n-1} - Z_1     & \ldots & Z_2 - Z_1 \\
			\vdots        & \vdots            & \ldots & 0         \\
			Z_n - Z_{n-2} & Z_{n_1} - Z_{n-2} & \ldots & 0         \\
			Z_n - Z_{n-1} & 0                 & \ddots & 0         \\
			0             & 0                 & \ldots & 0
		\end{bmatrix}
	\]
	As a result, we may write the dual problem compactly as
	\begin{equation}\label{eq:1d-dual-compact}
		\begin{aligned}
			d(\eta)
			 & =  \half \norm{\eta - y}_2^2 + \half \norm{y}^2_2                                         \\
			 & \hspace{2em} \text{ s.t. } \abr{\eta, 1} = 0, \norm{\eta [A_1, A_2]}_\infty \leq \lambda.
		\end{aligned}
	\end{equation}
	We recognize \cref{eq:1d-dual-compact} as the dual of a Lasso problem with
	weight matrix \( \sbr{A_1; A_2} \).
	Indeed, it is straightforward to directly calculate that the bi-dual problem is
	\begin{equation}
		\min_{v} \half \norm{[A_1; A_2] v + b - y} + \lambda \norm{v}_2,
	\end{equation}
	where the \( \ell_1 \) penalty comes from the conjugate of the \( \ell_\infty \)-norm
	constraint and the bias stems from the \( \eta^\top \mathbbm{1} = 0 \)
	constraint.

	Now, observe that \( \eta = 0 \) strictly satisfies the constraint in \cref{eq:1d-dual-compact},
	Slater's constraint qualification holds, and strong duality attains.
	Thus, the bidual has the same optimal value as the dual program.
	\citet{pilanci2020convexnn} show that strong duality holds for the
	original non-convex training problem and its dual as long as \( m \geq m^* \).
	Thus, the bidual attains the same optimal value as
	\cref{eq:1d-relu} under this condition.

	It remains only to check the mapping between solutions of the bidual and the original
	non-convex program preserves objective values.
	This is straightforward to do by direct calculation.
\end{proof}

\begin{lemma}
	Consider the one-dimensional training problem in \cref{eq:1d-relu}
	and assume that all examples \( Z_i \) are distinct.
	Then the optimal neural network is p-unique when \( n = 2 \) or \( n = 3 \).
\end{lemma}
\begin{proof}
	First consider \( n = 2 \).
	In this case, the data matrix for the corresponding lasso problem is given
	by
	\[
		A =
		\begin{bmatrix}
			0         & Z_2 - Z_1 \\
			Z_2 - Z_1 & 0
		\end{bmatrix},
	\]
	which is square and full rank. Thus, the lasso problem admits a unique
	solution and the optimal neural network is p-unique.

	The proof is slightly more complicated for \( n = 3 \).
	The data matrix is
	\[
		A =
		\begin{bmatrix}
			0         & 0         & Z_3 - Z_1 & Z_2 - Z_1 \\
			Z_2 - Z_1 & 0         & Z_3 - Z_2 & 0         \\
			Z_3 - Z_1 & Z_3 - Z_2 & 0         & 0
		\end{bmatrix},
	\]
	We check for uniqueness by checking if the columns of \( A \) are in
	general position, which is known to be a sufficient condition for
	uniqueness \citep{tibshirani2013unique}.
	The columns of \( A \) are in general position if and only if
	there do not exist \( n+1 \) columns of \( A \)
	and signs \( s_i \in \cbr{+1, -1} \) such that
	\[
		s_j a_j \in \text{Aff} \rbr{\cbr{s_i a_i}_{i \in \calI \setminus j}},
	\]
	for any choice of \( j \in \calI \).
	It is straightforward to show this holds by direct calculation.

	Consider \( j = 4 \).
	Inclusion in the affine hull requires
	\[
		s_1 (Z_2 - Z_1) = \alpha_3 s_3 (Z_3 - Z_1),
	\]
	which implies \( s_1 = s_3 \) and \( \alpha_3 = \frac{Z_2 - Z_1}{Z_3 - Z_1} \).
	Similarly,
	\begin{align*}
		0
		 & = \alpha_1 s_1 (Z_2 - Z_1) + \alpha_3 s_3 (Z_3 - Z_2)                    \\
		 & = \alpha_1 s_1 (Z_2 - Z_1) + s_3 (Z_3 - Z_2) \frac{Z_2 - Z_1}{Z_3 - Z_1} \\
		 & = (\alpha_1 s_1 + s_3 \frac{Z_3 - Z_2}{Z_3 - Z_1}) (Z_2 - Z_1),
	\end{align*}
	which implies \( s_1 = - s_3 \) and \( \alpha_1 = \frac{Z_3 - Z_2}{Z_3 - Z_1} \).
	Now, observe that
	\[
		\alpha_1 + \alpha_3 = \frac{Z_3 - Z_2}{Z_3 - Z_1} + \frac{Z_2 - Z_1}{Z_3 - Z_1} = 1,
	\]
	so that \( \alpha_2 = 0 \) is required.
	Since \( Z_3 - Z_2 \neq Z_3 - Z_1 \) because the \( Z_i \) are distinct,
	we conclude that the affine inclusion does not hold.
	Arguing in this manner for each choice of column gives the result.
\end{proof}

\begin{conjecture}
	The solution is not p-unique for \( n \geq 4 \).
\end{conjecture}
\begin{proof}
	I'm not certain how to show this result.
	For general data values, it turns into a combinatorial problem over (i)
	which $n = 4$ vectors to select out of the five possible and (ii) what
	signs $s_i$ to choose.
\end{proof}

\begin{lemma}
    
\end{lemma}
