# Supplementary material for: Optimal Sets and Solution Paths of ReLU Networks
Source: arXiv:2306.00119 source file (2024-01-19)
Supplement: Supplementary file 3 [file discontinuity.tex]

%!TEX root=../main.tex

% \oneNeuron*
\begin{proof}
	\citet{mishkin2022convex} show that \autoref{eq:relu-least-squares} has the same global optimal values as
	\begin{equation*}
		\min_{v, \gamma \in \cbr{-1, 1}} \half \norm{\sum_{i=1}^p (X v_i)_+ \gamma - y} + \lambda \sum_{i = 1}^p \norm{w_i}_2,
	\end{equation*}
	with objective-preserving mapping \( w_i = v_i / \sqrt{\norm{v_i}_2} \),
	\( \alpha_i = \gamma_i \sqrt{\norm{v_i}_2} \).
	Thus, we shall analyze this equivalent problem when characterizing \( s(\lambda) \).

	Consider the case \( p = 1 \).
	Let \( X, y \) consist of two training points, \( (x_1, y_1) = (-100, 1) \) and \( (x_2, y_2) = (1, 10) \).
	In what follows, we drop the subscript for \( v \) and \( \gamma \) since \( p = 1 \) and we consider a one-dimensional.
	The optimization problem of interest is
	\begin{equation*}
		\min_{v, \gamma} \half \rbr{(x_1 v)_+ \gamma - y_1}^2 + \rbr{(x_2 v)_+ \gamma - y_2}^2 + \lambda \abs{v}.
	\end{equation*}
	Since \( x_1 < 0 \) and \( x_2 > 0 \), we can re-write this optimization problem as
	\[
		\min_{v, \gamma} \half \mathbbm{1}_{v \leq 0} \rbr{\rbr{x_1 v \gamma - y_1}^2 + y_2^2} + \mathbbm{1}_{v > 0}\rbr{\rbr{x_2 v \gamma - y_2}^2 + y_1^2} + \lambda \abs{v}.
	\]
	By inspection, we see that \( \gamma = +1 \) is optimal in both cases, leading to the following simplified expression:
	\[
		\min_{v} \half \mathbbm{1}_{v \leq 0} \rbr{\rbr{x_1 v - y_1}^2 + y_2^2} + \mathbbm{1}_{v > 0}\rbr{\rbr{x_2 v - y_2}^2 + y_1^2} + \lambda \abs{v}.
	\]
	This is a piece-wise continuous (but non-smooth) quadratic with a breakpoint at \( v^* = 0 \).
	We not determine the solution to this minimization problem via a case analysis.

	\textbf{Case 1}: \( v^* = 0 \).
	Then, the optimal objective is trivially \( f(v^*) = y_1^2 + y_2^2 \).

	\textbf{Case 2}: \( v^* < 0 \).
	First order optimality conditions are
	\[
		x_1 \rbr{x_1 v_{-}^* - y_1} - \lambda = 0 \implies v_{-1}^* = \frac{y_1 \cdot x_1 + \lambda}{x_1^2},
	\]
	which is valid only if \( \lambda < |y_1 \cdot x_1| = 100 \).
	The minimum objective value is then
	\begin{align*}
		\half \rbr{\rbr{x_1 v_{-}^* - y_1}^2 + y_2^2} - \lambda v_{-}^*
		 & = \rbr{\rbr{x_1 \frac{y_1 \cdot x_1 + \lambda}{x_1^2} - y_1}^2 + y_2^2} - \lambda \rbr{\frac{y_1 \cdot x_1 + \lambda}{x_1^2}} \\
		 & = \frac{\lambda^2}{x_1^2} + y_2^2 - \lambda \rbr{\frac{y_1 \cdot x_1 + \lambda}{x_1^2}}                                       \\
		 & = -\frac{\lambda y_1}{x_1} + y_2^2.
	\end{align*}

	\textbf{Case 3}: \( v_{+}^* > 0 \).
	Similarly to the previous case, we obtain
	\[
		x_2 \rbr{x_2 v_{+}^* - y_2} + \lambda = 0 \implies v_{+}^* = \frac{y_2 \cdot x_2 - \lambda}{x_2^2},
	\]
	which is valid only if \( \lambda < |y_2 \cdot x_2| = 10 \).
	In this case, the minimum objective is
	\begin{align*}
		\half \rbr{\rbr{x_2 v_{+}^* - y_2}^2 + y_1^2} + \lambda v_{+}^*
		 & = \rbr{\rbr{x_2 \frac{y_2 \cdot x_2 + \lambda}{x_2^2} - y_2}^2 + y_1^2} - \lambda \rbr{\frac{y_2 \cdot x_2 + \lambda}{x_2^2}} \\
		 & = \frac{\lambda^2}{x_2^2} + y_2^2 + \lambda \rbr{\frac{y_2 \cdot x_2 - \lambda}{x_2^2}}                                       \\
		 & = \frac{\lambda y_2}{x_2} + y_1^2.
	\end{align*}

	To combine the cases, observe that
	\begin{align*}
		f(v_+^*) - f(v_-^*)
		 & = \frac{\lambda y_2}{x_2} + y_1^2 - \sbr{-\frac{\lambda y_1}{x_1} + y_2^2} \\
		 & = \lambda \rbr{\frac{x_1 y_2 + x_2 y_1}{x_1 x_2}} + y_1^2 - y_2^2          \\
		 & = \lambda \rbr{\frac{-100 (10) + 1 (1)}{-100 (1)}} + 1 - 100               \\
		 & = 9.99 \lambda - 99.
	\end{align*}
	We deduce that \( f(v_+^*) - f(v_-^*) > 0 \) (and thus \( v^* \leq 0 \))
	whenever \( \lambda > 9.90990991 \approx 10 \).

	In particular, taking \( \lambda = 10 \), we find
	\[
		f(v_-^*) = 100 - 0.1 = 99.99 < 101 = y_1^2 + y_2^2 = f(0),
	\]
	so that \( v_-^* \) is optimal and \( s(10) = v_-^* < 0 \).
	Moreover, \( v_-^* \) is strictly decreasing as a function of \( \lambda \),
	for all \( \lambda > 9.90990991 \)
	so that \( v_-^* \)

	Now, consider \( \lambda = 9.90990991 - \epsilon \) to see that
	\[
		f(v_+^*) = 100.0990991 - 10 \epsilon < 101 = y_1^2 + y_2^2 = f(0),
	\]
	for all \( \epsilon > 0 \).
	We deduce that \( v_+^* > 0 \) is optimal for all \( \epsilon > 0 \) and
	thus \( s(\lambda) \) is discontinuous at \( \lambda = 9.90990991 \).
\end{proof}
